# Supplementary material for: Training Constrained Deconvolutional Networks for Road Scene Semantic Segmentation
Source: arXiv:1604.01545 source file (2016-04-06)
Supplement: Supplementary file 1 [file appendix.tex]

\newpage
\appendix
\section{Supplementary Material} 
\label{app:AppendixA}

Images are initially normalized using spatial contrast normalization, independently applied to each channel $f$ as $\bar{X}_{i,j,f} = X_{i,j,f} / (1 + \alpha  \frac{1}{k^2}\sum_{j'=0}^{k-1}{\sum_{i'=0}^{k-1}{x^2_{i+i',j+j',f}}})^\beta$. Here $k=7$ stands for the kernel size and $\alpha = 1, \ \beta=0.5$.

\begin{table*}[]
	\centering
	\caption{Semantic segmentation quantitative results on the testing dataset, training with the Sparse domain.}
	\vspace{-3mm}
	%\resizebox{\textwidth}{!}{%
		\scriptsize
		\tabcolsep=0.06cm
		\begin{tabular}{@{}lcccccccc@{}}
			\toprule
			Method    & other & pole & car & sign & pedestrian & cyclist & \textbf{per-class} & \textbf{global} \\ \midrule
			FCN  	  & 94.1 & 1.0 & 92.8 & 10.8 & 77 & 77.5 & 58.9 & 93.1\\ \midrule
			P-Net     & 86.9 & 0 & 81.3 & 11.5 & 80 & 56.8     & 52.8 & 85.7\\ \bottomrule
		\end{tabular}%
	%}
	\label{tab:sparse_results}
\end{table*}

\begin{table*}[]
	\centering
	\caption{Evaluation of Knowledge Transference to P-Nets of different sizes.}
	\vspace{-3mm}
	\resizebox{\textwidth}{!}{%
		\scriptsize
		\tabcolsep=0.06cm
		\begin{tabular}{@{}lccccccccccccc@{}}
			\toprule
			Method    & sky & building & road & sidewalk & fence & vegetation & pole & car & sign & pedestrian & cyclist & \textbf{per-class} & \textbf{global} \\ \midrule
			T-Net $\rightarrow$ P-Net 6B (Probs)   & 87.3   	& 75.7     & 87.4   & 28.1      & 9.4     & 83.8    & 6.8    & 89.4   & 24.5    & 55.4         & 6.1      & 50.3                  & 75.3\\ \midrule               

			T-Net $\rightarrow$ P-Net 8B (Probs)       & 85.1   	& 65.1     & 87.5   & 21.1      & 35.7     & 85.3    & 6.6   & 90.0   & 45.2    & 53.2         & 55.6     & 57.3                 & 70.8               \\ \midrule

			T-Net $\rightarrow$ P-Net 10B (Probs)   & 84.1   	& 79.9     & 84.9   & 31.0      & 22.9     & 78.7    & 3.1    & 88.6   & 31.0    & 51.6         & 15.3      & 51.9                 & 75.7 \\ \midrule              
			\midrule
			T-Net $\rightarrow$ P-Net 6B (Probs-drop)   & 87.3   	& 75.7     & 87.4   & 28.1      & 9.4     & 83.8    & 6.8    & 89.4   & 24.5    & 55.4         & 6.1      & 50.3                  & 75.3\\ \midrule               

			T-Net $\rightarrow$ P-Net 8B (Probs-drop)   & 87.6   	& 75.9     & 79.3   & 43.2      & 27.1     & 80.8    & 4.0    & 86.9   & 19.9    & 68.5         & 14.0      & 53.4                  & 74.8\\ \midrule            

			T-Net $\rightarrow$ P-Net 10B (Probs-drop)   & 84.1   	& 79.9     & 84.9   & 31.0      & 22.9     & 78.7    & 3.1    & 88.6   & 31.0    & 51.6         & 15.3      & 51.9                 & 75.7 \\ \midrule              

		\end{tabular}%
	}
	\label{tab:multiblock}
\end{table*}
